# Supplementary material for: The statistical mechanics of complex signaling networks : nerve growth factor signaling
Source: arXiv:q-bio/0406043 source file (2004-06-22)
Supplement: Supplementary file 1 [file brown_supp.pdf]

# Supporting Online Material

## The Model

The mathematical model consists of a set of nonlinear ordinary differential equations (ODEs). Most chemicals (i. e. proteins) cycle between an inactive (dephosphorylated, phosphorylated, or GDP–bound) state and an active (phosphorylated, dephosphorylated, or GTP–bound) state, and conversions between these forms are facilitated by other signaling molecules in the network. All GTPase activating proteins (GAPs) and phosphatases in the network are assumed static. Other than EGF, NGF, and their respective receptors (Huff et al., 1981; Yankner and Shooter, 1979), we lack good data for absolute chemical concentrations in the network. We therefore assume all active (signaling–competent) concentrations are initially at zero to avoid signal transmission in the absence of growth factor stimulation. All inactive signaling molecules are assumed to be at a starting concentration of 1 $\mu$M, except for Mek and Erk which are assumed to be fivefold more abundant. EGF and NGF concentrations were converted from ng/ml to number of molecules/cell using a cell diameter of 20 $\mu$m and experimental conditions of 5 ml media volume in 60 mm dishes. Typical experimental EGF and NGF concentrations used are far into the saturating regime, so we expect the model output to be relatively insensitive to the details of this conversion. The parameters that are allowed to fluctuate in the meta–model are are the $k$'s and $K_m$'s. The ODEs were integrated with a fifth order Runge–Kutta–type method (Press et al., 1996). The complete set of equations for the model shown in Fig. 1 follows; to obtain the equations for the model lacking PI3K, all terms and equations involving active and inactive PI3K and Akt are removed, resulting in a set of equations with four fewer signaling molecules and eight fewer rate constants.

$$\frac{d\,[\mathrm{EGF}]}{dt} = -k_{\mathrm{rbEGF}}\,[\mathrm{EGF}]\,[\mathrm{freeEGFReceptor}]$$

$$
\begin{aligned}
& +k_{\mathrm{ruEGF}}\,[\mathrm{boundEGFReceptor}] \\
\frac{d\,[\mathrm{NGF}]}{dt} &= -k_{\mathrm{rbNGF}}\,[\mathrm{NGF}]\,[\mathrm{freeNGFReceptor}] \\
& +k_{\mathrm{ruNGF}}\,[\mathrm{boundNGFReceptor}] \\
\frac{d\,[\mathrm{freeEGFReceptor}]}{dt} &= -k_{\mathrm{rbEGF}}\,[\mathrm{EGF}]\,[\mathrm{freeEGFReceptor}] \\
& +k_{\mathrm{ruEGF}}\,[\mathrm{boundEGFReceptor}] \\
\frac{d\,[\mathrm{boundEGFReceptor}]}{dt} &= +k_{\mathrm{rbEGF}}\,[\mathrm{EGF}]\,[\mathrm{freeEGFReceptor}] \\
& -k_{\mathrm{ruEGF}}\,[\mathrm{boundEGFReceptor}] \\
\frac{d\,[\mathrm{freeNGFReceptor}]}{dt} &= -k_{\mathrm{rbNGF}}\,[\mathrm{NGF}]\,[\mathrm{freeNGFReceptor}] \\
& +k_{\mathrm{ruNGF}}\,[\mathrm{boundNGFReceptor}] \\
\frac{d\,[\mathrm{boundNGFReceptor}]}{dt} &= +k_{\mathrm{rbNGF}}\,[\mathrm{NGF}]\,[\mathrm{freeNGFReceptor}] \\
& -k_{\mathrm{ruNGF}}\,[\mathrm{boundNGFReceptor}] \\
\frac{d\,[\mathrm{SosInactive}]}{dt} &= -k_{\mathrm{EGF}}\,[\mathrm{boundEGFReceptor}]\,\frac{[\mathrm{SosInactive}]}{[\mathrm{SosInactive}]+K_{\mathrm{mEGF}}} \\
& -k_{\mathrm{NGF}}\,[\mathrm{boundNGFReceptor}]\,\frac{[\mathrm{SosInactive}]}{[\mathrm{SosInactive}]+K_{\mathrm{mNGF}}} \\
& +k_{\mathrm{dSos}}\,[\mathrm{P90RskActive}]\,\frac{[\mathrm{SosActive}]}{[\mathrm{SosActive}]+K_{\mathrm{mdSos}}} \\
\frac{d\,[\mathrm{SosActive}]}{dt} &= +k_{\mathrm{EGF}}\,[\mathrm{boundEGFReceptor}]\,\frac{[\mathrm{SosInactive}]}{[\mathrm{SosInactive}]+K_{\mathrm{mEGF}}} \\
& +k_{\mathrm{NGF}}\,[\mathrm{boundNGFReceptor}]\,\frac{[\mathrm{SosInactive}]}{[\mathrm{SosInactive}]+K_{\mathrm{mNGF}}} \\
& -k_{\mathrm{dSos}}\,[\mathrm{P90RskActive}]\,\frac{[\mathrm{SosActive}]}{[\mathrm{SosActive}]+K_{\mathrm{mdSos}}} \\
\frac{d\,[\mathrm{P90RskInactive}]}{dt} &= -k_{\mathrm{pP90Rsk}}\,[\mathrm{ErkActive}]\,\frac{[\mathrm{P90RskInactive}]}{[\mathrm{P90RskInactive}]+K_{\mathrm{mpP90Rsk}}} \\
\frac{d\,[\mathrm{P90RskActive}]}{dt} &= +k_{\mathrm{pP90Rsk}}\,[\mathrm{ErkActive}]\,\frac{[\mathrm{P90RskInactive}]}{[\mathrm{P90RskInactive}]+K_{\mathrm{mpP90Rsk}}} \\
\frac{d\,[\mathrm{RasInactive}]}{dt} &= -k_{\mathrm{Sos}}\,[\mathrm{SosActive}]\,\frac{[\mathrm{RasInactive}]}{[\mathrm{RasInactive}]+K_{\mathrm{mSos}}}
\end{aligned}
$$

$$
\begin{aligned}
& +k_{\mathrm{RasGap}} \left[\mathrm{RasGapActive}\right] \frac{\left[\mathrm{RasActive}\right]}{\left[\mathrm{RasActive}\right] + K_{\mathrm{mRasGap}}} \\
\frac{d\left[\mathrm{RasActive}\right]}{dt} &= +k_{\mathrm{Sos}} \left[\mathrm{SosActive}\right] \frac{\left[\mathrm{RasInactive}\right]}{\left[\mathrm{RasInactive}\right] + K_{\mathrm{mSos}}} \\
& -k_{\mathrm{RasGap}} \left[\mathrm{RasGapActive}\right] \frac{\left[\mathrm{RasActive}\right]}{\left[\mathrm{RasActive}\right] + K_{\mathrm{mRasGap}}} \\
\frac{d\left[\mathrm{RasGapActive}\right]}{dt} &= 0
\end{aligned}
$$

$$
\begin{aligned}
\frac{d\left[\mathrm{Raf1Inactive}\right]}{dt} &= -k_{\mathrm{RasToRaf1}} \left[\mathrm{RasActive}\right] \frac{\left[\mathrm{Raf1Inactive}\right]}{\left[\mathrm{Raf1Inactive}\right] + K_{\mathrm{mRasToRaf1}}} \\
& +k_{\mathrm{dRaf1}} \left[\mathrm{Raf1PPtase}\right] \frac{\left[\mathrm{Raf1Active}\right]}{\left[\mathrm{Raf1Active}\right] + K_{\mathrm{mdRaf1}}} \\
& +k_{\mathrm{dRaf1ByAkt}} \left[\mathrm{AktActive}\right] \frac{\left[\mathrm{Raf1Active}\right]}{\left[\mathrm{Raf1Active}\right] + K_{\mathrm{mRaf1ByAkt}}} \\
\frac{d\left[\mathrm{Raf1Active}\right]}{dt} &= +k_{\mathrm{RasToRaf1}} \left[\mathrm{RasActive}\right] \frac{\left[\mathrm{Raf1Inactive}\right]}{\left[\mathrm{Raf1Inactive}\right] + K_{\mathrm{mRasToRaf1}}} \\
& -k_{\mathrm{dRaf1}} \left[\mathrm{Raf1PPtase}\right] \frac{\left[\mathrm{Raf1Active}\right]}{\left[\mathrm{Raf1Active}\right] + K_{\mathrm{mdRaf1}}} \\
& -k_{\mathrm{dRaf1ByAkt}} \left[\mathrm{AktActive}\right] \frac{\left[\mathrm{Raf1Active}\right]}{\left[\mathrm{Raf1Active}\right] + K_{\mathrm{mRaf1ByAkt}}} \\
\frac{d\left[\mathrm{BRafInactive}\right]}{dt} &= -k_{\mathrm{Rap1ToBRaf}} \left[\mathrm{Rap1Active}\right] \frac{\left[\mathrm{BRafInactive}\right]}{\left[\mathrm{BRafInactive}\right] + K_{\mathrm{mRap1ToBRaf}}} \\
& +k_{\mathrm{dBRaf}} \left[\mathrm{Raf1PPtase}\right] \frac{\left[\mathrm{BRafActive}\right]}{\left[\mathrm{BRafActive}\right] + K_{\mathrm{mdBRaf}}} \\
\frac{d\left[\mathrm{BRafActive}\right]}{dt} &= +k_{\mathrm{Rap1ToBRaf}} \left[\mathrm{Rap1Active}\right] \frac{\left[\mathrm{BRafInactive}\right]}{\left[\mathrm{BRafInactive}\right] + K_{\mathrm{mRap1ToBRaf}}} \\
& -k_{\mathrm{dBRaf}} \left[\mathrm{Raf1PPtase}\right] \frac{\left[\mathrm{BRafActive}\right]}{\left[\mathrm{BRafActive}\right] + K_{\mathrm{mdBRaf}}} \\
\frac{d\left[\mathrm{MekInactive}\right]}{dt} &= -k_{\mathrm{pRaf1}} \left[\mathrm{Raf1Active}\right] \frac{\left[\mathrm{MekInactive}\right]}{\left[\mathrm{MekInactive}\right] + K_{\mathrm{mpRaf1}}} \\
& -k_{\mathrm{pBRaf}} \left[\mathrm{BRafActive}\right] \frac{\left[\mathrm{MekInactive}\right]}{\left[\mathrm{MekInactive}\right] + K_{\mathrm{mpBRaf}}} \\
& +k_{\mathrm{dMek}} \left[\mathrm{PP2AActive}\right] \frac{\left[\mathrm{MekActive}\right]}{\left[\mathrm{MekActive}\right] + K_{\mathrm{mdMek}}} \\
\frac{d\left[\mathrm{MekActive}\right]}{dt} &= +k_{\mathrm{pRaf1}} \left[\mathrm{Raf1Active}\right] \frac{\left[\mathrm{MekInactive}\right]}{\left[\mathrm{MekInactive}\right] + K_{\mathrm{mpRaf1}}}
\end{aligned}
$$

$$
\begin{aligned}
& +k_{\mathrm{pBRaf}}\,[\mathrm{BRafActive}]\,\frac{[\mathrm{MekInactive}]}{[\mathrm{MekInactive}]+K_{\mathrm{mpBRaf}}} \\
& -k_{\mathrm{dMek}}\,[\mathrm{PP2AActive}]\,\frac{[\mathrm{MekActive}]}{[\mathrm{MekActive}]+K_{\mathrm{mdMek}}} \\
\frac{d\,[\mathrm{ErkInactive}]}{dt} &= -k_{\mathrm{pMek}}\,[\mathrm{MekActive}]\,\frac{[\mathrm{ErkInactive}]}{[\mathrm{ErkInactive}]+K_{\mathrm{mpMek}}} \\
& +k_{\mathrm{dErk}}\,[\mathrm{PP2AActive}]\,\frac{[\mathrm{ErkActive}]}{[\mathrm{ErkActive}]+K_{\mathrm{mdErk}}} \\
\frac{d\,[\mathrm{ErkActive}]}{dt} &= +k_{\mathrm{pMek}}\,[\mathrm{MekActive}]\,\frac{[\mathrm{ErkInactive}]}{[\mathrm{ErkInactive}]+K_{\mathrm{mpMek}}} \\
& -k_{\mathrm{dErk}}\,[\mathrm{PP2AActive}]\,\frac{[\mathrm{ErkActive}]}{[\mathrm{ErkActive}]+K_{\mathrm{mdErk}}} \\
\frac{d\,[\mathrm{PI3KInactive}]}{dt} &= -k_{\mathrm{PI3K}}\,[\mathrm{boundEGFReceptor}]\,\frac{[\mathrm{PI3KInactive}]}{[\mathrm{PI3KInactive}]+K_{\mathrm{mPI3K}}} \\
& -k_{\mathrm{PI3KRas}}\,[\mathrm{RasActive}]\,\frac{[\mathrm{PI3KInactive}]}{[\mathrm{PI3KInactive}]+K_{\mathrm{mPI3KRas}}} \\
\frac{d\,[\mathrm{PI3KActive}]}{dt} &= +k_{\mathrm{PI3K}}\,[\mathrm{boundEGFReceptor}]\,\frac{[\mathrm{PI3KInactive}]}{[\mathrm{PI3KInactive}]+K_{\mathrm{mPI3K}}} \\
& +k_{\mathrm{PI3KRas}}\,[\mathrm{RasActive}]\,\frac{[\mathrm{PI3KInactive}]}{[\mathrm{PI3KInactive}]+K_{\mathrm{mPI3KRas}}} \\
\frac{d\,[\mathrm{AktInactive}]}{dt} &= -k_{\mathrm{Akt}}\,[\mathrm{PI3KActive}]\,\frac{[\mathrm{AktInactive}]}{[\mathrm{AktInactive}]+K_{\mathrm{mAkt}}} \\
\frac{d\,[\mathrm{AktActive}]}{dt} &= +k_{\mathrm{Akt}}\,[\mathrm{PI3KActive}]\,\frac{[\mathrm{AktInactive}]}{[\mathrm{AktInactive}]+K_{\mathrm{mAkt}}} \\
\frac{d\,[\mathrm{C3GInactive}]}{dt} &= -k_{\mathrm{C3GNGF}}\,[\mathrm{boundNGFReceptor}]\,\frac{[\mathrm{C3GInactive}]}{[\mathrm{C3GInactive}]+K_{\mathrm{mC3GNGF}}} \\
\frac{d\,[\mathrm{C3GActive}]}{dt} &= +k_{\mathrm{C3GNGF}}\,[\mathrm{boundNGFReceptor}]\,\frac{[\mathrm{C3GInactive}]}{[\mathrm{C3GInactive}]+K_{\mathrm{mC3GNGF}}} \\
\frac{d\,[\mathrm{Rap1Inactive}]}{dt} &= -k_{\mathrm{C3G}}\,[\mathrm{C3GActive}]\,\frac{[\mathrm{Rap1Inactive}]}{[\mathrm{Rap1Inactive}]+K_{\mathrm{mC3G}}} \\
& +k_{\mathrm{RapGap}}\,[\mathrm{RapGapActive}]\,\frac{[\mathrm{Rap1Active}]}{[\mathrm{Rap1Active}]+K_{\mathrm{mRapGap}}} \\
\frac{d\,[\mathrm{Rap1Active}]}{dt} &= +k_{\mathrm{C3G}}\,[\mathrm{C3GActive}]\,\frac{[\mathrm{Rap1Inactive}]}{[\mathrm{Rap1Inactive}]+K_{\mathrm{mC3G}}} \\
& -k_{\mathrm{RapGap}}\,[\mathrm{RapGapActive}]\,\frac{[\mathrm{Rap1Active}]}{[\mathrm{Rap1Active}]+K_{\mathrm{mRapGap}}}
\end{aligned}
$$

$$\frac{d\,[\mathrm{RapGapActive}]}{dt} = 0$$

$$\frac{d\,[\mathrm{PP2AActive}]}{dt} = 0$$

$$\frac{d\,[\mathrm{Raf1PPtase}]}{dt} = 0$$

**Additional Data**

Time series data for a variety of signaling molecules (those with a solid border in Fig. 1) were obtained from seven sources (chu Kao et al., 2001; Traverse et al., 1992; Qiu and Green, 1991; Yao et al., 1995; York et al., 1998; Traverse et al., 1994). Because of differences in data for Erk1/2 phosphorylation obtained from several sources (Traverse et al., 1992; Yao et al., 1995; Traverse et al., 1994), we used multiple Erk1/2 phosphorylation data sets simultaneously in ensemble generation rather than picking one set. Our cost function requires error bars, but some published data sets have either no error bars or error bars whose determination is unclear. We therefore assign a relative error of 20% to data sets lacking error bars and make very small errors equal to 10% relative. This procedure incorporates our lack of knowledge about the method of error determination while not penalizing researchers who have gone to the trouble to estimate errors in their data. We obtain similar results from the model whether we use the quoted errors in the data or the procedure described above, so we are confident that our manipulation of the experimental errors is benign. Figures S1 through S7 show all the experimental data used and the corresponding model output. The ensemble used in these figures is the same used to generate figures 2 and 4 in the main manuscript.

**Differentiation Assays**

PC12 cells were grown in RPMI 1640 (Cellgro) supplemented with 10% horse serum and 5% calf serum (both Gibco) to subconfluency (40-50%) in six-well tissue culture plates coated with 10 $\mu$g/cm type VII rat–tail collagen (Sigma). 16 hours prior to growth factor treatments, media was changed to RPMI 1640 with 1% calf serum. Fresh low serum media was added every other day. EGF at 100 ng/ml and NGF at 50 ng/ml (both Gibco) were added every other day. LY 294002 (Calbiochem) at a concentration of 10 $\mu$M was added every day. On days when LY and growth factors were both added, LY was added at least 2 hours prior to growth factor treatment. Cells were scored for neurite extensions after 2 and 4 days, and the results in table S1 represent an average over 3 independent experiments ($\pm$ S. D. ). At least 450 cells in multiple fields were counted to obtain the percentages in table S1. Samples treated with LY alone did not differentiate, but not enough cells were viable on days 2 and 4 to obtain proper counts.

# REFERENCES

chu Kao, S., R. K. Jaiswal, W. Kolch, and G. E. Landreth. 2001. Identification of the mechanisms regulating the differential activation of the MAPK cascade by epidermal growth factor and nerve growth factor in PC12 cells. *J. Biol. Chem.* 276:18169–18177.

Huff, K., D. End, and G. Guroff. 1981. Nerve growth factor–induced alteration in the response of PC12 pheochromocytoma cells to epidermal growth factor. *J. Cell Biol.* 88:189–198.

Press, W. H., S. A. Teukolsky, W. T. Vetterling, and B. P. Flannery. 1996. Numerical Recipes in C. Cambridge University Press, New York, second edition.

Qiu, M.-S. and S. H. Green. 1991. NGF and EGF rapidly activate p21Ras in PC12 cells by distinct, convergent pathways involving tyrosine phosphorylation. *Neuron* 7:937–946.

Traverse, S., N. Gomez, H. Paterson, C. Marshall, and P. Cohen. 1992. Sustained activation of the mitogen-activated protein (MAP) kinase cascade may be required for differentiation of PC12 cells. *Biochem. J.* 288:351–355.

Traverse, S., K. Seedorf, H. Paterson, C. J. Marshall, P. Cohen, and A. Ullrich. 1994. EGF triggers neuronal differentiation of PC12 cells that overexpress the EGF receptor. *Curr. Biol.* 4:694–701.

Yankner, B. and E. M. Shooter. 1979. Nerve growth factor in the nucleus : interaction with receptors on the nuclear membrane. *Proc. Natl. Acad. Sci. USA* 76:1269–1273.

Yao, H., K. Labudda, C. Rim, P. Caodieci, M. Loda, and P. J. S. Stork. 1995. Cyclic adenosine monophosphate can convert epidermal growth factor into a differentiating factor in neuronal cells. *J. Biol. Chem.* 270:20748–20753.

York, R. D., H. Yao, T. Dillon, C. L. Ellig, S. P. Eckert, E. W. McClesky, and P. J. S. Stork. 1998. Rap1 mediates sustained MAP kinase activation induced by nerve growth factor. *Nature* 392:622–626.

| Treatment | 2 Days | 4 Days |
|---|---|---|
| 0 | $1.6 \pm 0.9$ | $5 \pm 2$ |
| EGF | $4.8 \pm 0.7$ | $8.9 \pm 0.5$ |
| NGF | $32 \pm 5$ | $48 \pm 7$ |
| EGF + LY | $6.3 \pm 0.8$ | $8 \pm 1$ |
| NGF + LY | $23 \pm 3$ | $35 \pm 3$ |

**Table S1.** Results of PC12 differentiation assay. Ligand/LY concentrations and experimental protocol are as described above. Data is reported as percent differentiated (mean) $\pm$ S. D.

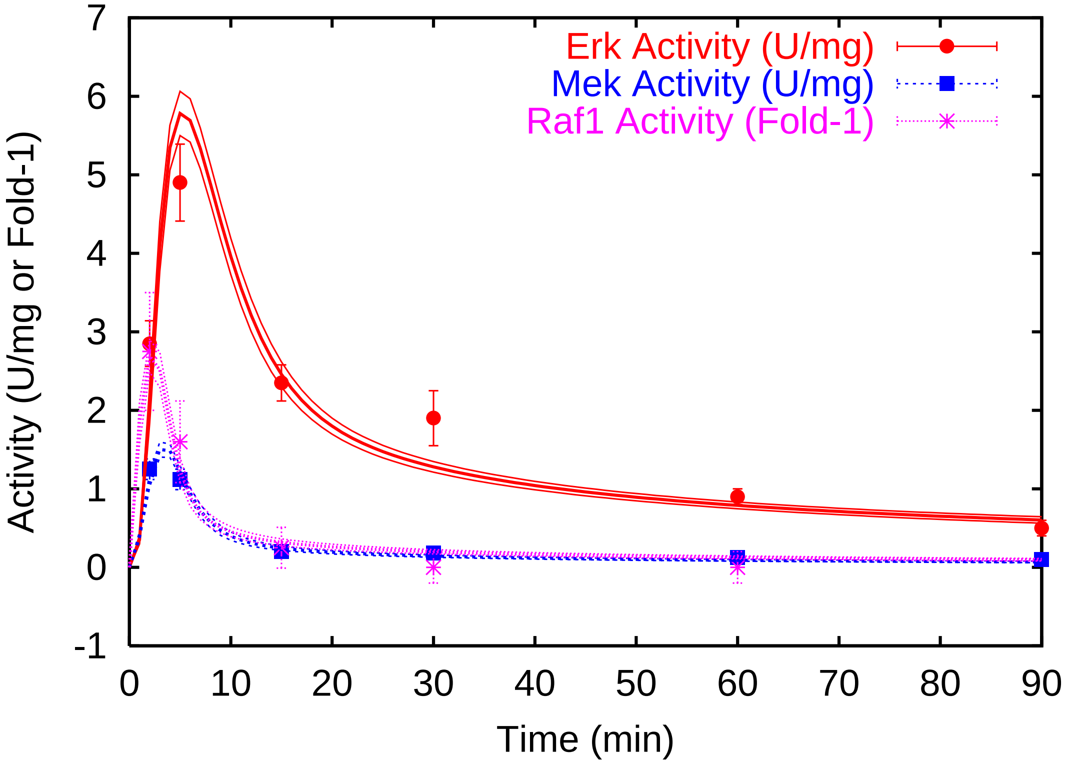


**Figure S1.** Data and model behavior for EGF stimulation of 100 ng/ml. Experimental data was taken from references (chu Kao et al., 2001) and (Traverse et al., 1994). This figure and S2–S7 show all the data simultaneously used for Hessian calculation and ensemble generation. In this and the six subsequent figures experimental data and errors are represented by points with error bars and model mean and one sigma deviations are given by the solid curves, with the central darker curve representing the mean. In each case, the legend shows which signaling molecule is associated with which color curves and data points, which match so one can easily see which curves correspond to which data points.

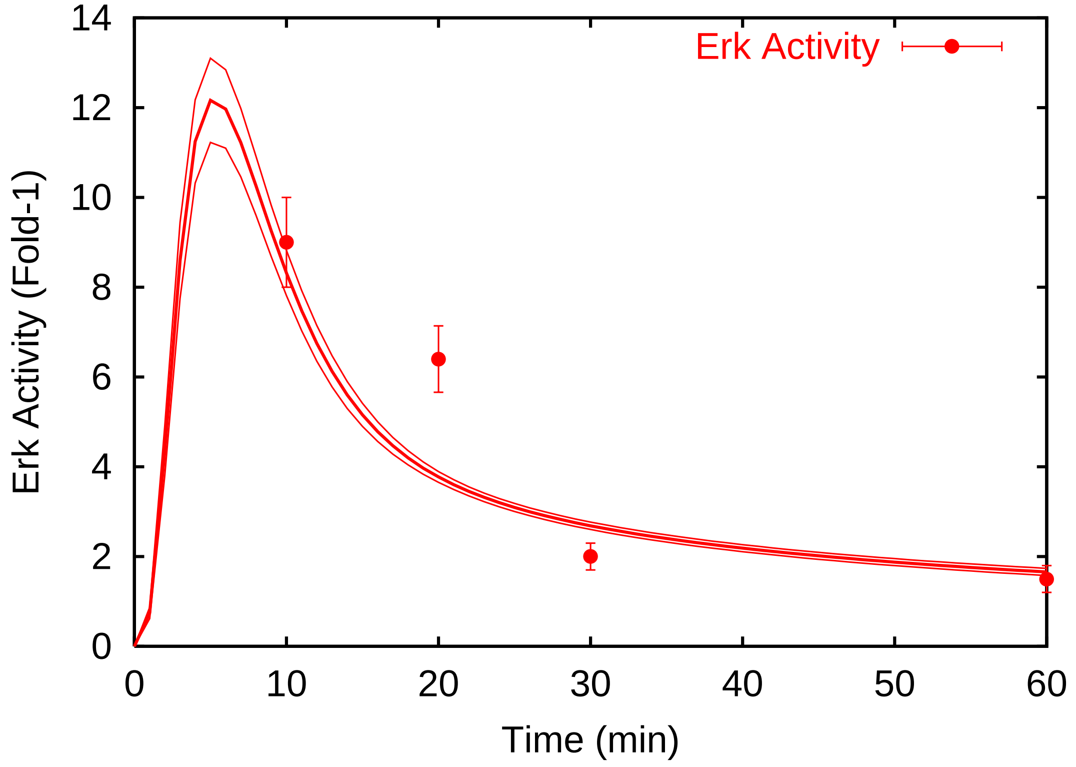


**Figure S2.** Data and model behavior for EGF stimulation of 100 ng/ml. Experimental data was taken from reference (Yao et al., 1995).

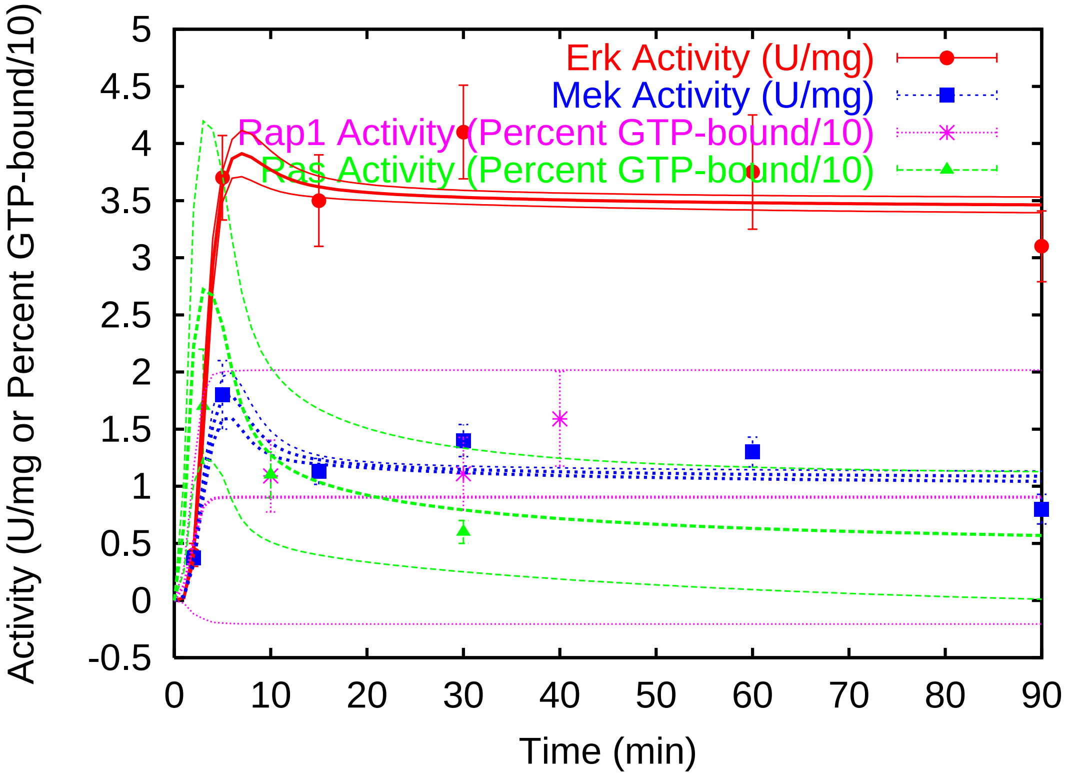


**Figure S3.** Data and model behavior for NGF stimulation at 50 ng/ml. Experimental data was taken from references (Yao et al., 1995),(York et al., 1998), and (Qiu and Green, 1991). Error curves for active Rap1 (pink) and active Ras (green) are larger than typical in the other figures because both molecules do not need B factors (see Equation 1 in the main paper); they are measured in terms of percent binding GTP, which is calculable based on knowing the active and total concentrations of each in the model. The entropic contribution of the $B_k$ factors balances cost penalties for deviation from these data sets, and we expect this phenomenon when we use thermal sampling for any model that mixes time series with $B_k$ factors and those without.

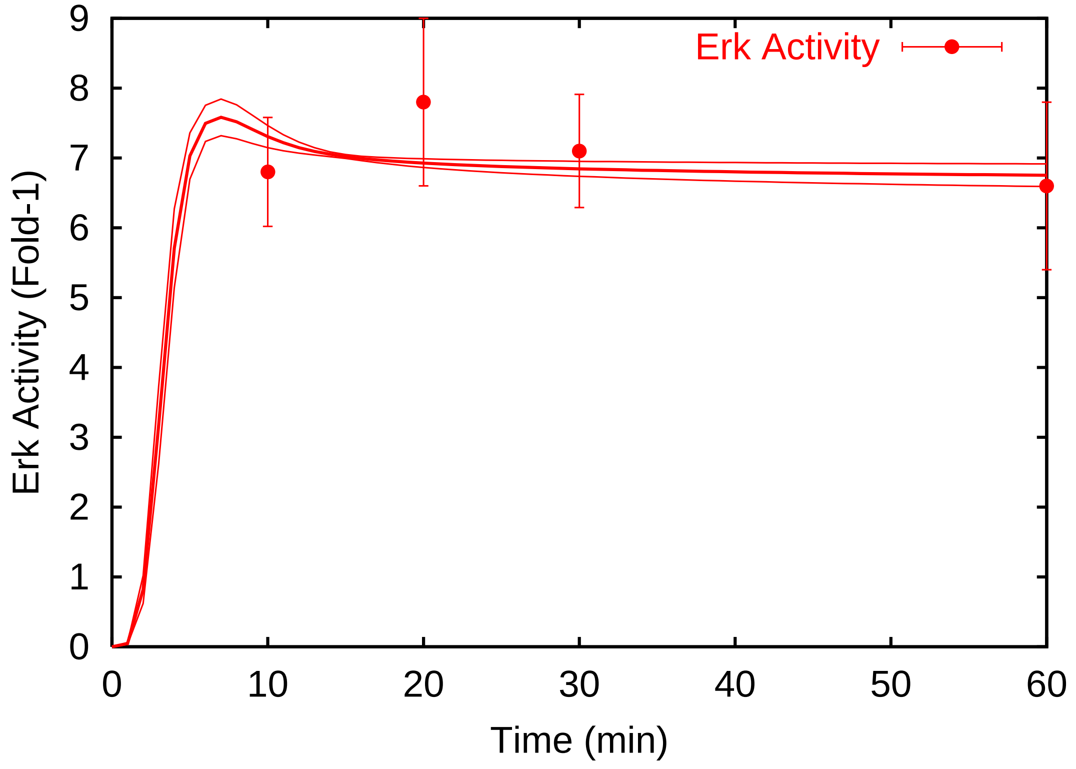


**Figure S4.** Data and model behavior for NGF stimulation at 50 ng/ml. Experimental data is that of reference (Yao et al., 1995).

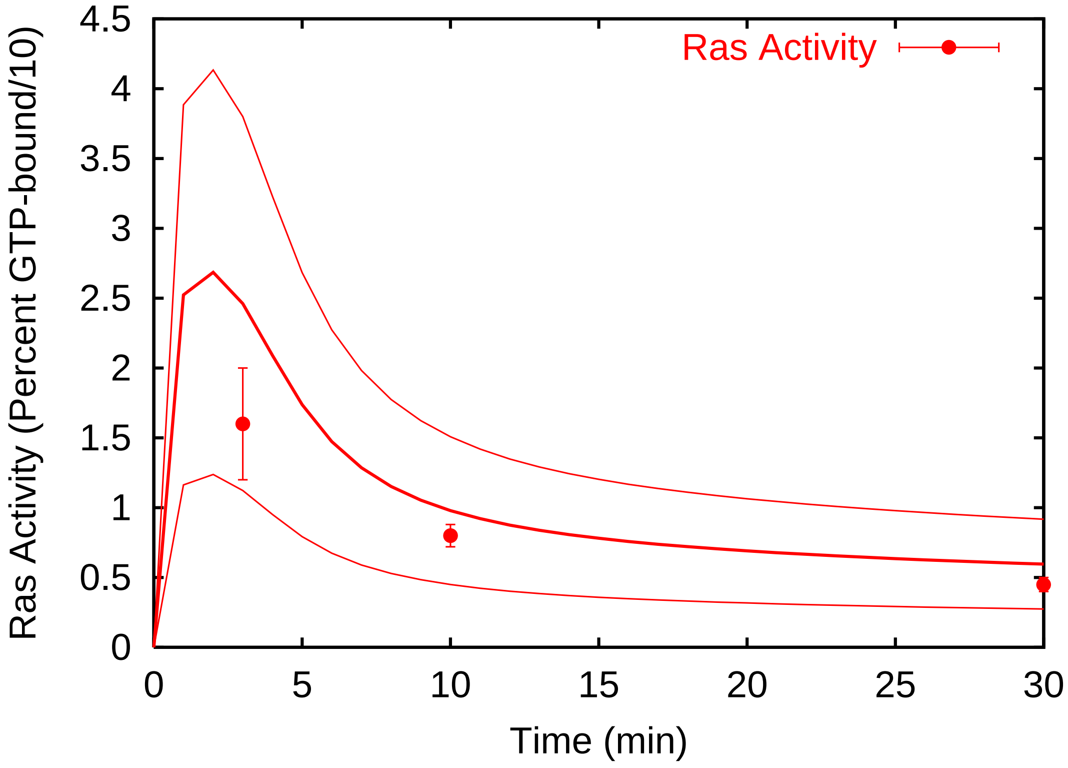


**Figure S5.** Data and model behavior for EGF stimulation at 30 ng/ml. Experimental data comes from reference (Qiu and Green, 1991). The larger than typical size of the model error curves are for the reasons explained in Figure S3.

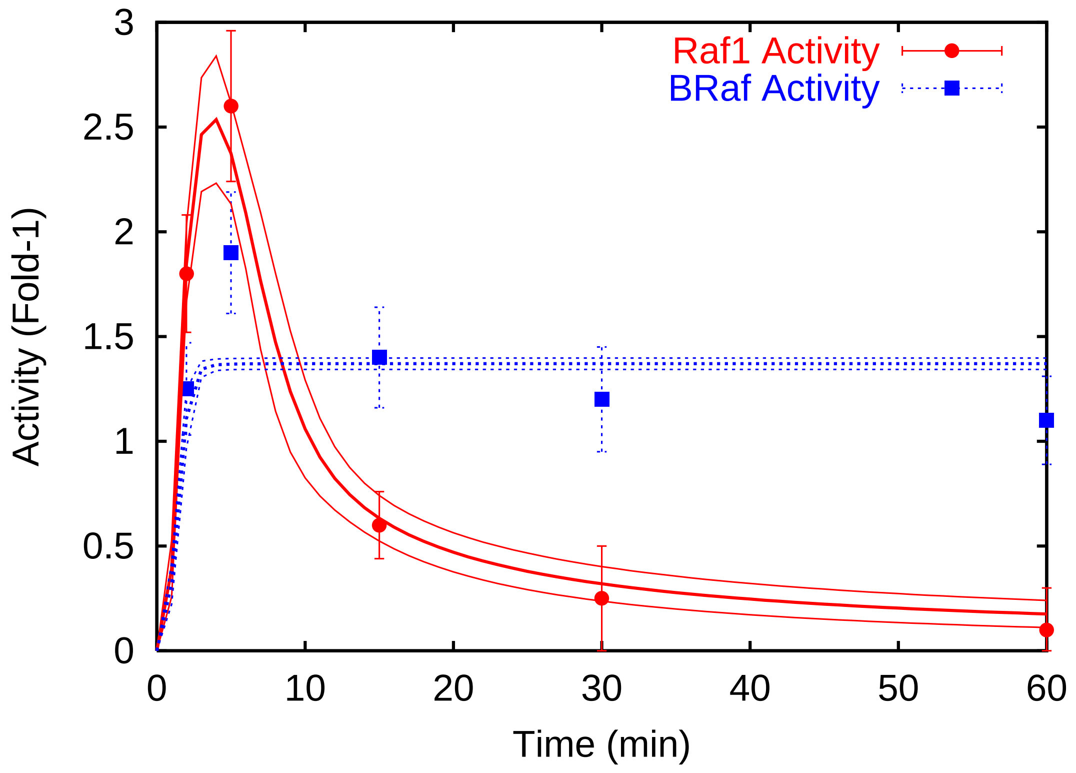


**Figure S6.** Data and model behavior for NGF stimulation at 100 ng/ml. Data is that of reference (chu Kao et al., 2001).

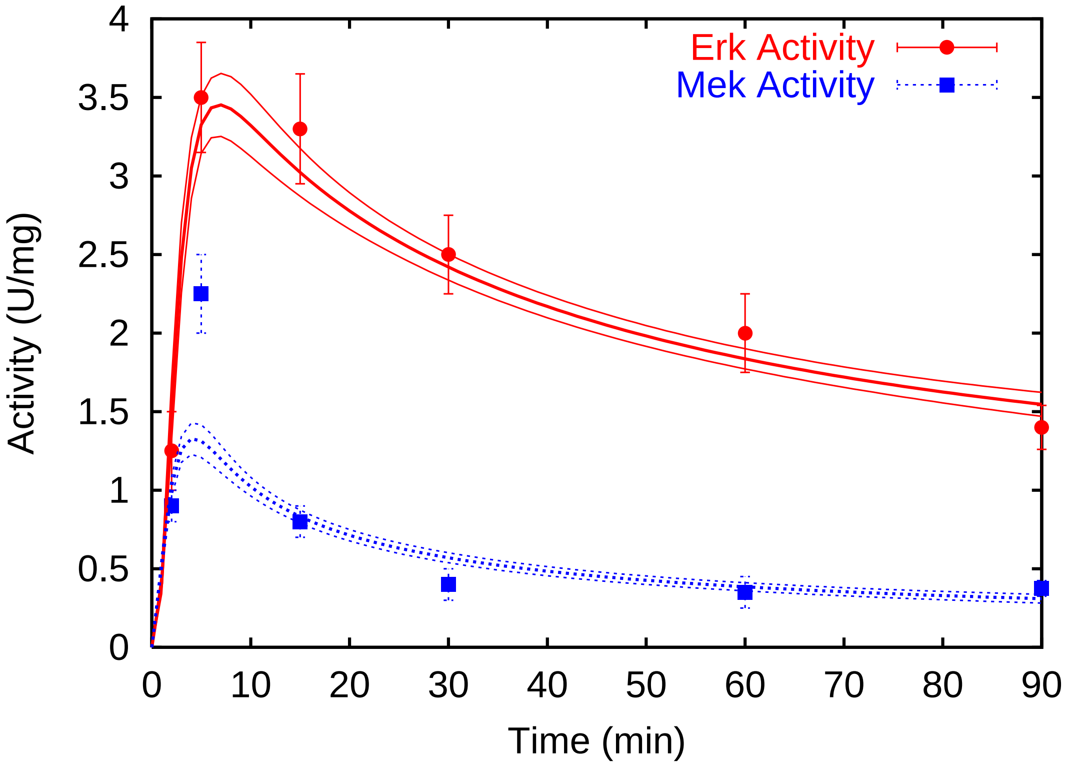


**Figure S7.** Data and model behavior for EGF stimulation at 100 ng/ml when the EGFR is overexpressed 50–fold. Experimental data is that of reference (Traverse et al., 1994).
